# Supplementary material for: Handling Spatial-Temporal Data Heterogeneity for Federated Continual Learning via Tail Anchor
Source: arXiv:2412.18355 source file (2025-03-05)
Supplement: Supplementary file 1 [file X_suppl.tex]

\clearpage
\setcounter{page}{1}
\appendix
\maketitlesupplementary

\section{Algorithm}
\label{Alogrithm}
Please see \autoref{alo1}.

\begin{algorithm*}[htbp]
\caption{FedTA Algorithm.}
\label{alo1}
  % \SetAlgoLined
  \KwIn{$a$ clients $\mathcal{A} = \{A_i\}_{i=1}^a$ with their own task sequence $\mathcal{T}_i = \{T_i^n\}_{n=1}^N$, a pre-trained frozen ViT $\mathcal{V}$ without classification head, a pre-set threshold $Thres$ for measuring similarity.}
  
  \KwOut{Fused global input enhancement knowledge base $\mathcal{KB}_G$, best global prototypes $\mathcal{P}_G$ with the lowest average similarity.}
  % \BlankLine
  
  Initialization\;
  \While{task number n $\leq$ N}{
        \For{each client $A_i, 1 \leq i \leq a$}{
        
        $\mathcal{V}_e^i$ $\gets$ \rm{LoadHead}(${H}_e^i,\mathcal{V}$)\;
        
        \rm{\textbf{Stage 1: Training \textit{Input Enhancement}:}}
        
        \For{each $\{x, y\} \in T_i^n$}{
        $E$ $\gets$ \rm{EmbeddingLayer}($x$)\;

        $\{{K}^{ie}_{chosen},IE_{chosen}\}$ $\gets$ \rm{QueryforInputEnhancement ($E,\mathcal{V},\mathcal{KB}_{i}$)\; \tcp{Key-value pair.}}

        $E'$ $\gets$ \rm{concatenation}($E,IE_{chosen}$)\;

        $\mathcal{L}_{ce}$ $\gets$ \rm{Classify}($\mathcal{V}_g^i,E',y$) \;\tcp{Classification loss with $\mathcal{V}_e^i$.}

        \rm{Optimize}($\mathcal{L}_{ce},{H}_e^i,{K}^{ie}_{chosen},IE_{chosen}$)\; \tcp{\autoref{loss1}.}

        }
        \rm{\textbf{Freeze \textit{Input Enhancement};}}
         
        \rm{\textbf{Stage 2: Training \textit{Tail Anchor}:}}

        \For{each $\{x, y\} \in T_i^n$}{

        $E'$ $\gets$ \rm{GetInputEnhancement}($x,\mathcal{KB}_i,\mathcal{V}$)\;
        
        $\{{K}^{ta}_{chosen},TA_{chosen}\}$ $\gets$ \rm{QueryforTailAnchor}($\mathcal{TA}_i,E',\mathcal{V}_e^i$);

         $\mathcal{F}_{TA}$ $\gets$ \rm{MixFeatureWithTailAnchor}($\mathcal{V}_e^i(x),TA_{chosen}$)\;

        $L_{ce}$ $\gets$ \rm{Classify}($\mathcal{F}_{TA},y$)\;

         \If{$\mathcal{P}^g$ is not none}{
            $L_{cons}$ $\gets$ \rm{ContrastiveLearning}($\mathcal{P}^g,\mathcal{F}_{TA}$)\;\tcp{\autoref{loss2}.}
         }

        \rm{Optimize}($\mathcal{L}_{CE},\mathcal{L}_{cons},\mathcal{H}_e^i,{K}^{ta}_{chosen},TA_{chosen}$)\;
        }
        
        \rm{\textbf{Freeze \textit{Tail Anchor};}}
        
        $\mathcal{P}_i$ $\gets$ \rm{ComputerLocalPrototype}($\mathcal{T}_i^n,\mathcal{TA}_i,\mathcal{KB}_i,\mathcal{V}_e^i$) \;
        }

        \rm{\textbf{Server aggregation:}}
        
        \rm{\textbf{For \textit{Input Enhancement:}}}
        
        $\mathcal{KB}_G$ $\gets$ \rm{SelectivePromptFusion}($\mathcal{KB}_1,\mathcal{KB}_2,\ldots,\mathcal{KB}_a$) \;

        \rm{\textbf{For \textit{Local Prototypes:}}}

        $\mathcal{M}$ $\gets$ \rm{SimilarityAdjacentMatrix}($\mathcal{P}_1,\mathcal{P}_2,\ldots,\mathcal{P}_a$)\;
        \For{each class Y in $\mathcal{T}^n$}{

        $(P^Y_G,Simi^Y)$ $\gets$ \ \rm{FindLowestAvergeSimilarity}($\mathcal{M},Y$)\;

        \If{$Simi^Y$ $\leq Thres$}{
            \rm{FixGlobalPrototype}($P^Y_G$)\; \tcp{The global prototype of class Y will not be changed again.}
        }

        Add $P^Y_G$ into $\mathcal{P}_G$\;
            
        }

        \textbf{Distribute $\mathcal{P}_G$ and $\mathcal{KB}_G$ to all clients for next task training.}
    }
\end{algorithm*}

\section{Experiments setting}
\label{setting}

\subsection{Datasets} 
We conduct extensive experiments on CIFAR-100 \cite{krizhevsky2009learning} and ImageNet-R \cite{hendrycks2021many} with 5 incremental tasks to evaluate the effectiveness of our FedTA in addressing spatial-temporal catastrophic forgetting. CIFAR-100 is a widely used benchmark dataset and consists of 60,000 RGB color images, each of size 32x32 pixels, classified into 100 different classes. The ImageNet-R dataset consists of 200 classes, containing 24,000 training samples and 6,000 testing samples. It is worth noting that ImageNet-R serves as a robust metric for evaluating the generalization capability of pre-trained models, and it is used to assess performance in continual learning methods \cite{wang2022dualprompt}.

\subsection{Implementation Details} 
In our setup, the federated system consists of five clients and one central server, and each client possesses a sequence of five tasks. We repeat experiments with three random seeds (42,1999,2024) and report the averaged outcomes. Across all methods, we fix the number of clients at five and the interval rounds for increments at five. We employ Adam as the optimizer with a learning rate of $0.001$. The whole training process is performed sequentially on an NVIDIA GPU RTX-3090.

\subsection{Baselines}

\textbf{FedAvg} \cite{mcmahan2017communication}: FedAvg is a fundamental algorithm in federated learning. It works by first distributing a global model to multiple clients. Each client trains the model locally using its own data for a few epochs. Then, the clients send their locally updated models back to a central server. The server aggregates these local models by computing their weighted average to update the global model. This process is repeated for several rounds until the global model converges.

\textbf{FedProx} \cite{li2020federated}: FedProx is an algorithm designed to address issues in federated learning, particularly the challenges of heterogeneous data and varying computational capabilities among clients. It extends the FedAvg algorithm by introducing a proximal term to the local objective function. This proximal term helps to keep local updates closer to the global model, reducing the impact of local model divergence.

\textbf{FedLwF} \cite{li2017learning}:LwF is a distillation-based method. Instead of unlabeled data, LwF leverages new task data to perform distillation. FedLwF denotes FedAvg with LwF applied to clients.

\textbf{GLFC} (Global Local Forgetting Compensation) \cite{dong2022federated}: a synchronous FCIL method. GLFC designs a class-aware gradient compensation loss and a class-semantic relation distillation loss to mitigate forgetting and distill consistent inter-class relations across tasks. A proxy server is implemented to select the optimal previous global model to assist the class-semantic relation distillation and a prototype gradient-based communication mechanism is developed to protect data privacy.

\textbf{TARGET} \cite{zhang2023target}: TARGET is an asynchronous Federated Class-Continual Learning method that effectively mitigates catastrophic forgetting by leveraging prior globally trained models for knowledge transfer at the model level and generating synthetic data to simulate the global data distribution at the data level. 

\textbf{MFCL} \cite{babakniya2024data}: MFCL (Mimicking Federated Continual Learning) leverages a generative model trained on the server to synthesize samples from past data distributions, which are then used alongside the training data to mitigate catastrophic forgetting. To preserve privacy, the generative model is trained by the server using data-free methods at the end of each task without requesting data from clients. 

\textbf{FedViT} \cite{dosovitskiy2020image}: a hybrid method of ViT and FedAvg. ViT segments the image into fixed-size small blocks, referred to as ``patches," and treats these patches as ``tokens" in a sequence, which are then fed into a Transformer encoder for processing. The global aggregation is performed by computing the average weights of the classification heads. 

\textbf{FedL2P} \cite{wang2022learning}: a hybrid method of L2P and FedAvg. L2P is a prompt-based CL method, which applies learnable task-specific prompts to mitigate forgetting.

\textbf{FedDualP} \cite{wang2022dualprompt}: a hybrid method of DualPrompt and FedAvg. DualPrompt, a prompt-based CL method derived from L2P, decouples the learnable prompts into general and expert prompts, encoding task-invariant and task-specific knowledge, respectively.

\textbf{FedNova} \cite{wang2020tackling}: normalizes the gradient weights to eliminate objective inconsistency of local training.

\textbf{FedMGP} \cite{yu2024personalized}: FedMGP takes into account the multi-granularity expression of knowledge, promoting the spatial-temporal integration of knowledge.

\textbf{Ours-w/o TA} refers to our method without \textit{Tail Anchor}. \textbf{Ours-w/o SIKF} refers to our method without \textit{Selective Input Knowledge Fusion}. \textbf{Ours-w/o BGPS} refers to our method without \textit{Best Global Prototype Selection}.

\begin{table*}[htbp]
\small
\begin{center}
\caption{Accuracy of the local model testing on local test sets.}
\label{result-appendix}
\begin{tabular}{cccccccccccc}
\toprule
\multirow{3}{*}{Algorithm}  &\multicolumn{5}{c}{CIFAR-100} & \multicolumn{5}{c}{Imagenet-R} \\
 &  \multicolumn{5}{c}{Task ID} & \multicolumn{5}{c}{Task ID} \\
 & 1& 2 & 3 & 4 & 5 & 1& 2 & 3 & 4 & 5 \\

\midrule
FedAvg\cite{mcmahan2017communication}   & 65.1 & 68.2 & 72.5 & 72.9 & 76.1 & 40.1 & 42.5 & 42.5 & 47.0 & 46.4   \\

% FedAvg+EWC &  &0.86 & 1.00 & 1.00 & 1.00 & 1.00 \\
FedProx\cite{li2020federated}  & 56.5 & 55.2 & 61.1 & 59.3 & 62.8 & 33.3  & 31.2 & 32.1 & 33.9 & 34.1 \\

GLFC\cite{dong2022federated} & 95.3 & 77.3 & 92.7 & 85.5 & 79.8 & 87.4 & 61.2 & 81.6 & 68.7 & 76.5 \\

FedLwF & 74.5 & 12.5 & 17.1 & 13.6 & 9.7 &34.3 &9.2 &2.6 &4.0 & 3.8 
 \\

TARGET\cite{zhang2023target}& 73.9 & 46.2 & 32.5 & 15.2 & 13.2 & 45.4 & 17.2 &17.4 & 19.1 & 18.6 \\ 

MFCL\cite{babakniya2024data} & 52.3 & 16.8 & 11.8 & 14.6 & 13.4&31.6 & 14.5 & 16.2 & 13.3 & 13.8 \\

\midrule
FedViT &  87.3 &87.1 &86.8 &86.4 &87.1 &80.0 & 74.7 & 74.1 &76.1 & 75.9 \\ 

FedL2P\cite{wang2022continual}  & 89.8 & 88.3 &72.2 &58.5 & 57.1 & 86.7 &84.6 &84.6 &86.7 &84.7\\

FedDualP\cite{wang2022dualprompt}  &76.4 & 75.8 & 74.9 & 73.9 & 75.9 & 65.7 & 61.8 &60.5 &60.6 & 61.8  \\
\midrule

Ours (FedTA) & 97.0 & 96.6 &96.6 &96.8 & 92.2& 81.7 & 80.5 & 80.1 &82.3 &85.9 \\
Ours-w/o TA & 81.7 & 78.5 & 78.7 & 77.7 & 77.0 	& 84.2 & 80.5 & 76.1 &80.5 &79.5 
 \\

Ours-w/o SIKF &91.5 & 91.5 & 92.2 & 92.0 & 92.1&83.3 &81.6 & 80.3&81.7&80.8 \\

Ours-w/o BGPS & 91.7 &93.3 & 90.5 & 92.8 & 92.9& 82.5 &79.1 & 81.5 & 83.1 &80.4 \\

\bottomrule
\end{tabular}
\vspace{-5mm}
\end{center}
\end{table*}

\section{Detailed Analysis of Fig.4}
\label{detail fig4}

Both on CIFAR-100 and on ImageNet-R, FedTA demonstrates satisfactory retention of spatial and temporal knowledge. Moreover, ablation experiments indicate that if the Tail Anchor component is removed, FedTA would also suffer from severe spatial-temporal catastrophic forgetting. The next best performer is FedViT, which, by freezing all parameters and leaving only a trainable classification head, can effectively overcome parameter-forgetting. However, the output-forgetting of the classification head is inevitable.

It is worth noting that although \textit{TARGET}, \textit{FedLwF} and \textit{MFCL} have achieved over 90\% in spatial knowledge retention, the accuracy of these methods' local models before aggregation was already quite low. Therefore, when compared to the accuracy after aggregation, it appears that the spatial knowledge retention is high. \autoref{result-appendix} displays the performance of the local models on their local test sets before aggregation, where FedTA still performs the best. Additionally, among the four novel components we designed, the \textit{Tail Anchor} has been proven by ablation experiments to be the most effective part, both in overcoming the negative impact of spatial-temporal data heterogeneity and in enhancing model performance.

\section{Detailed Analysis of Fig.5}
\label{detail fig5}

\begin{figure}[htbp]
  \centering
  \includegraphics[width=0.4\textwidth]{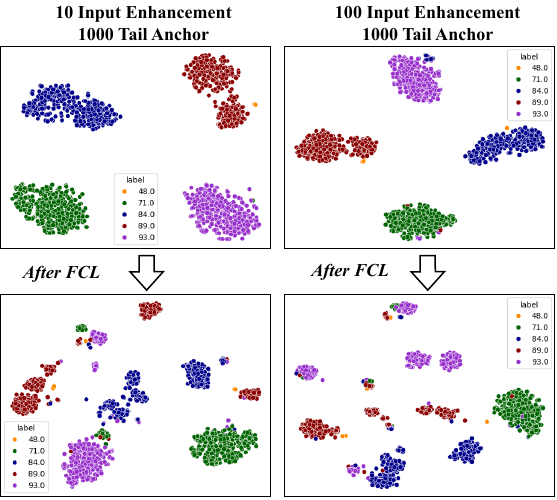}
  \vspace{-3mm}
  \caption{T-SNE for extra sensitivity analysis.}
  \vspace{-3mm}
  \label{sensitivity analysis-extra}
\end{figure}

Since the feature extractor of ViT is frozen, only \textit{Input Enhancement} and \textit{Tail Anchor} components affect the position of the features. Moreover, these two components are likely to be used by samples from different batches, leading to parameter-forgetting. Therefore, we conduct a sensitivity analysis on the number of these two components, attempting to find the optimal combination.

\autoref{sensitivity analysis} illustrates the changes in feature positions after FCL when different quantities of Input Enhancement and Tail Anchor are combined. When the number of Tail Anchors is set to 100, regardless of the quantity of Input Enhancements, the features of a portion of the data still deviate from their original positions. We speculate that this is due to the insufficient number of Tail Anchors, causing samples from the same class to match with completely dissimilar Tail Anchors. When we set the number of Tail Anchors to 500, the number of shifted points significantly decreases. The combination of 10 Input Enhancements and 500 Tail Anchors shows the most satisfactory visualization results.

We can hypothesize that it seems the more Tail Anchors there are, the fewer the number of shifted points, and the lower the probability of output-forgetting. However, when we set the number of Tail Anchors to 1000, as shown in \autoref{sensitivity analysis-extra}, it overturns our previous hypothesis. The number of shifted points is even greater and more disordered than when it was set to 100. We believe that this phenomenon occurs because the excessive number of Tail Anchors causes the matched Tail Anchor for the same sample to change constantly during the query function, preventing convergence to the best anchor point. 

\begin{table*}[!htbp]
\begin{center}
\setlength{\tabcolsep}{3pt}
\caption{Averaged accuracy of the global model on local test sets with 10 class-incremental tasks (CIFAR-100).}
\label{tab:cifar100-10}
\begin{tabular}{cccccccccccc|ccc}
\toprule
\multirow{2}{*}{Algorithm}  &\multirow{2}{*}{Type}&\multicolumn{10}{c}{Task ID} \\
 & & 1& 2 & 3 & 4 & 5 & 6 & 7 & 8 & 9 & 10 & $\overline{KR_t}$ &$\overline{KR_s}$ & Time (s) \\

\midrule
FedAvg & \multirow{3}{*}{FL} & 59.2 & 65.1 &	62.5 &	70.8 &	63.0 &	56.2 & 57.9 &	64.9 &	69.1 &	68.6  & 29.3\% & 83.1\% & 39878.76   \\

% FedAvg+EWC &  &0.86 & 1.00 & 1.00 & 1.00 & 1.00 \\
FedProx & &42.6 &	28.6 &	36.43 &	42.5 &	31.8 &	35.6 &	35.6 &	33.1 &	39.7 &	24.8 & 41.2\% &
55.7\% & 41214.89\\

FedNova & & 24.0 &	27.9 &	28.1 &	21.4 &	33.1 &	26.0 &	27.1 &	16.0 &	33.6 &	28.7 & 33.5\% & 42.6\% & 47507.69  \\

\midrule

FedLwF & \multirow{4}{*}{FL+CL} & 60.7 &	28.1 &	29.1 &	20.1 &	34.7 &	31.3 &	22.3 &	26.4 &	20.6 & 15.6 & 36.7\% &
87.0\% & 29716.53\\
FedViT & & 84.6 & 80.4 &	85.7 &	77.3 &	81.3 &	76.4 &	72.7 &	80.6 &	78.9 &	82.2 & 23.0\% & 94.8\% & 27718.24  \\ 

FedL2P & & 59.4 &	58.7 &	61.8 &	58.0&	49.1 &	52.8 &	56.1 &	63.8 & 52.5& 52.6 & 67.1\% & 60.5\% & 17894.10  \\

FedDualP &  & 62.4 &	77.1 &	67.2 &	66.6 &	63.9 &	42.5 &	60.8 &	46.4 & 64.4 &	64.7 & 22.0\% & 74.8\% & 68140.25
\\

\midrule

GLFC  & \multirow{5}{*}{FCL}& 44.3 & 61.7 &	89.5 &	77.4 &	85.9 &	63.6 &	74.5 &	78.5 &	81.9 &	82.7 & 64.5\% & 87.0\% & 61677.32 \\

TARGET & & 64.15 &	23.0 &	8.25 &	12.8 &	19.4 &	12.8 &	20.9 &	14.9 &	20.2 &	13.1 & 57.5\% & 82.0\% & 6676.68 \\ 

MFCL & &59.9 &	21.0 &	1.7 &	36.3 &	17.5 &	17.3 &	18.2 &	17.0 & 	21.5&	21.5&  67.2\% & 91.8\% & 38093.29\\

FedWEIT & &50.8 & 38.7&	32.6 &	39.4 &	43.4 &	37.0 &	45.9 & 44.9 &  37.7 & 53.2 &61.7\% & 65.9\% & 82324.58\\
FedSpace & & 47.7 &	55.7 &	54.2 &	45.3 &	48.3 &  56.8 & 46.2 & 53.2 &  47.3 & 58.2  &45.7\% & 79.9\% & 89324.88\\

\midrule

FedTA & FCL & 91.4& 	95.3 &	93.8 &	92.3 &	93.7 &	89.5 &	92.5 & 94.2 &	91.9 &	90.6 & 98.6\% & 99.8\%& 47013.82 \\

\bottomrule
\end{tabular}
\end{center}
\end{table*}

It is worth noting that compared to the output forgetting caused by traditional methods, FedTA has greatly alleviated the issue of output shifts caused by spatial-temporal changes, enabling it to overcome the negative impacts brought about by spatial-temporal data heterogeneity, namely, spatial-temporal catastrophic forgetting.

\section{Experiments with more tasks and extra baselines}
\label{extraresults}
There are a total of 3 clients, each with 25 private classes and 25 public classes, meaning each client has data from 50 classes. Each client performs 10 incremental tasks, with each task containing 5 classes. The data among clients and between tasks is non-overlapping, ensuring strong spatial-temporal data heterogeneity. Please note that in this scenario, we have only considered the situation with three clients, as the limitation of the CIFAR-100 does not ensure high spatial data heterogeneity with multiple clients. Such data distribution not only ensures strong data heterogeneity among clients but also maintains strong data heterogeneity between tasks. This presents a more challenging and, at the same time, more practically significant problem in combating both spatial and temporal forgetting. The final results indicate that FedTA not only surpasses other baseline methods on the two newly established metrics (i.e., Temporal Knowledge Retention and Spatial Knowledge Retention), but also achieves a significant improvement in accuracy. This implies that FedTA has successfully preserved local knowledge during the aggregation process, enabling the aggregated global model to perform so well on the local test sets.

To more intuitively illustrate the communication overhead and low training cost of FedTA, we have added a ``Training Time" column in the last column of the additional experimental results in \autoref{tab:cifar100-10}. This allows readers to more directly compare the advantages of different methods through training time. Below are the result of training time. From the results, it can be seen that compared to FedAvg, our method incurs a slightly higher cost in training time, primarily spent in the server's selective input knowledge fusion phase, as it involves knowledge distillation across multiple local models. However, compared to other FCL methods, our approach has reduced the training time.
